# Supplementary material for: How Well Do LLMs Identify Cultural Unity in Diversity?
Source: arXiv:2408.05102 source file (2024-08-09)
Supplement: Supplementary file 1 [file heatmap_of_culture.tex]

\begin{figure}[h]

\begin{center}
    \begin{minipage}{0.49\linewidth}
        \centering
        \includegraphics[width=1.0\linewidth]{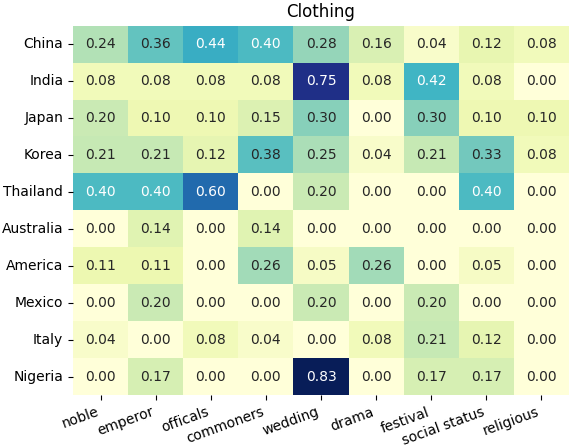}
    \end{minipage}
    %\qquad
    \begin{minipage}{0.49\linewidth}
        \centering
        \includegraphics[width=1.0\linewidth]{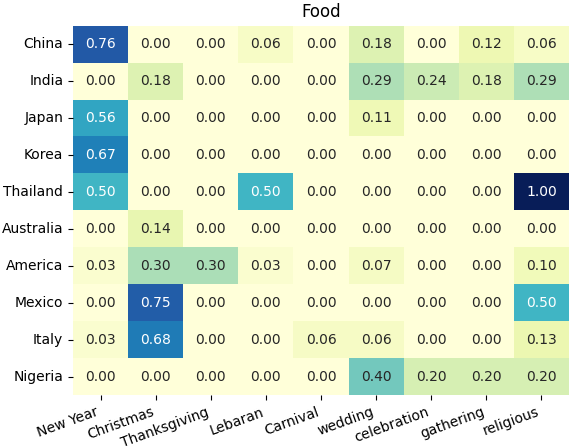}
    \end{minipage}
    \centering
\end{center}

\caption{\textbf{The results of some features in different geo-cultures.} We select the most frequent feature words in different geo-cultures and counted the frequency of feature occurrences of different cultural-specific concepts in different countries.}
\label{fig:heatmap_of_cultures}
\end{figure}
